# Supplementary material for: A complete description of P- and S-wave contributions to the $B^0\to K^{+}\pi^{-}\ell^{+}\ell^{-}$ decay
Source: arXiv:2107.05301 source file (2021-07-12)

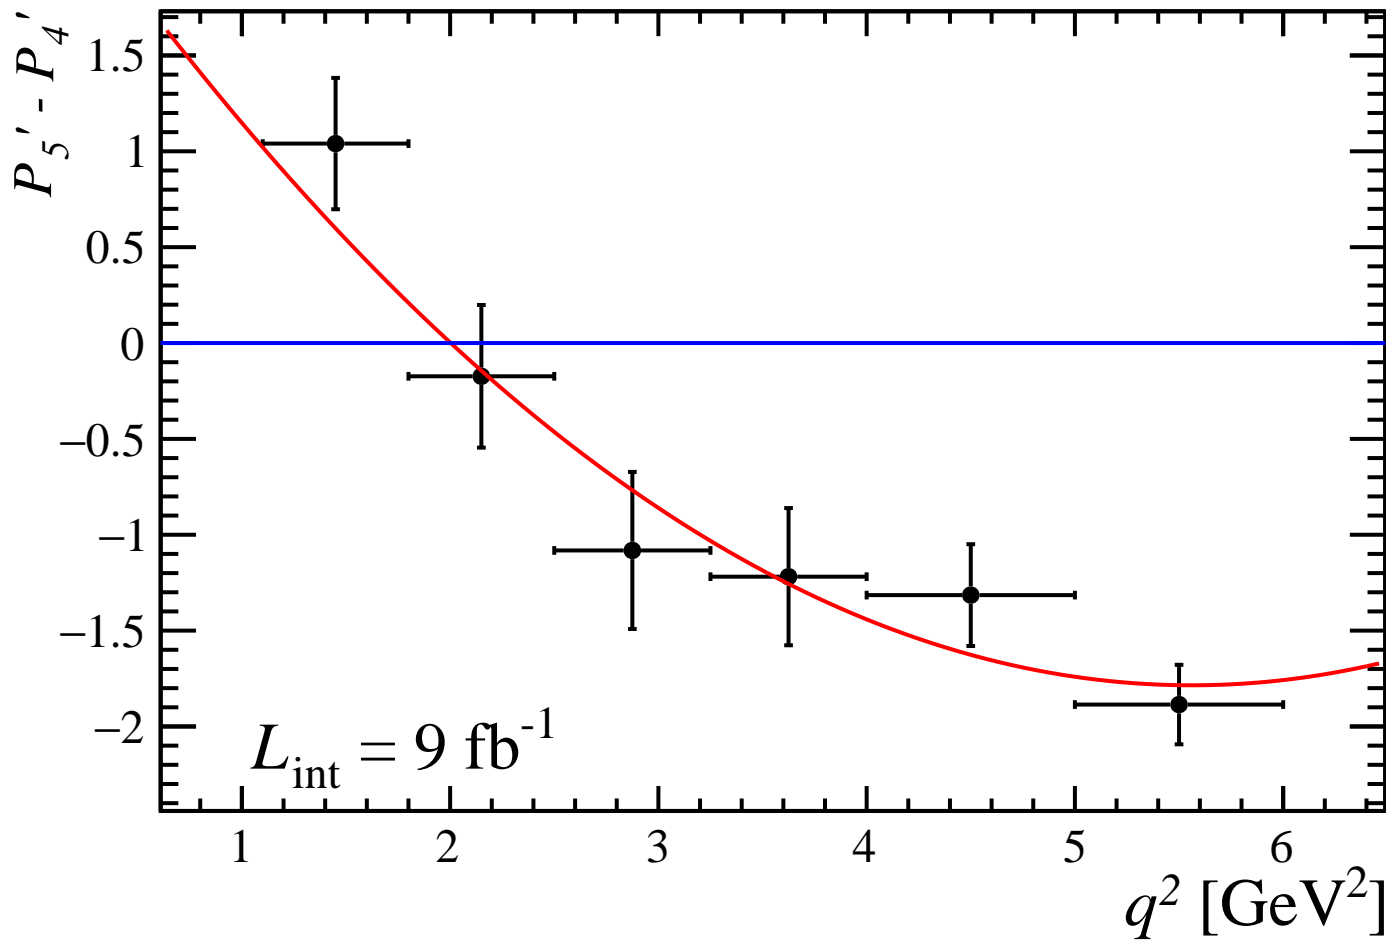

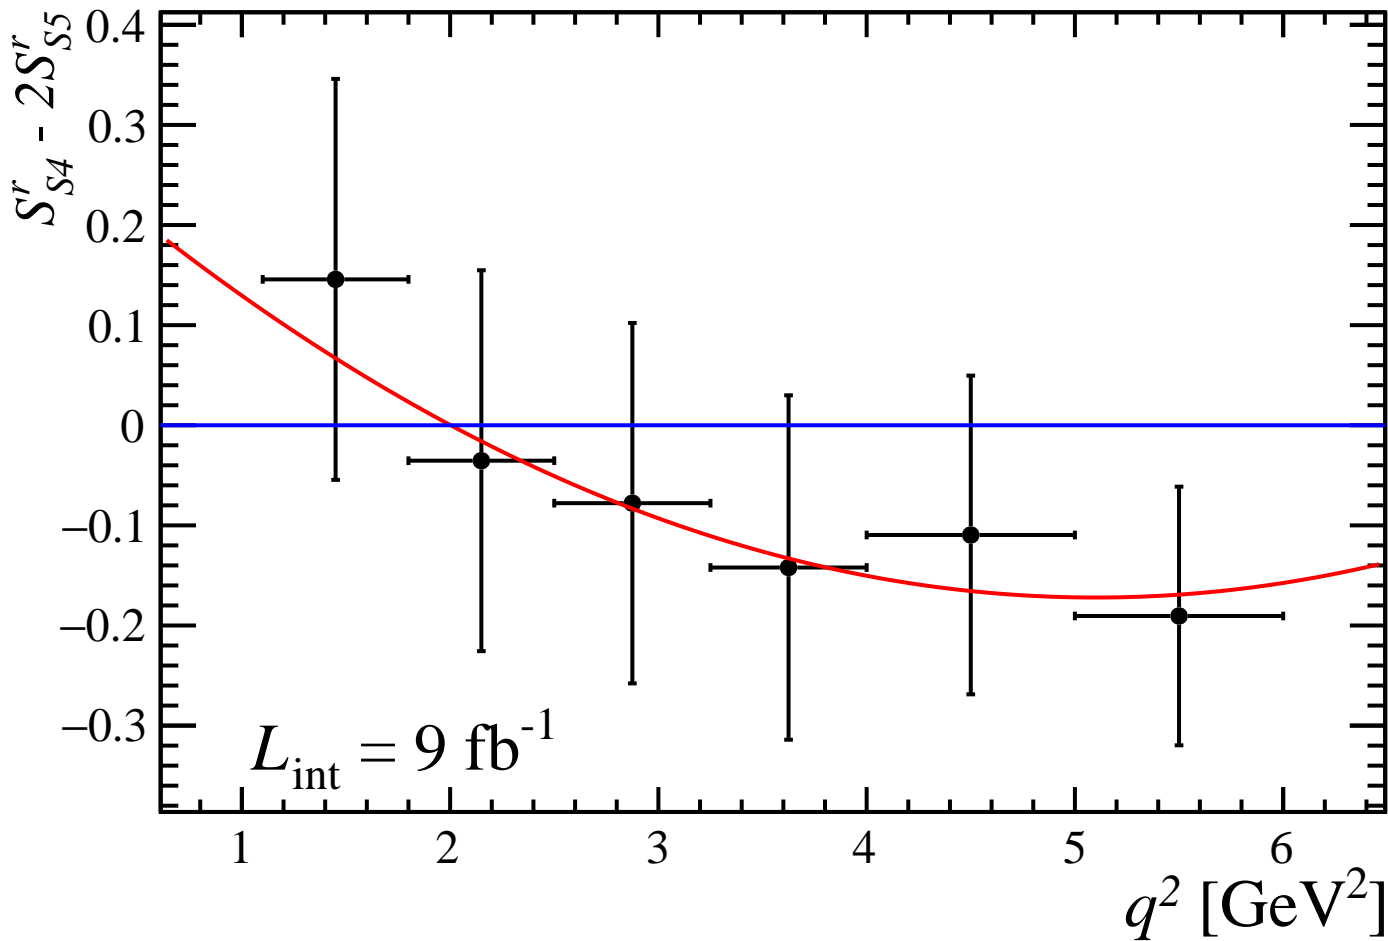

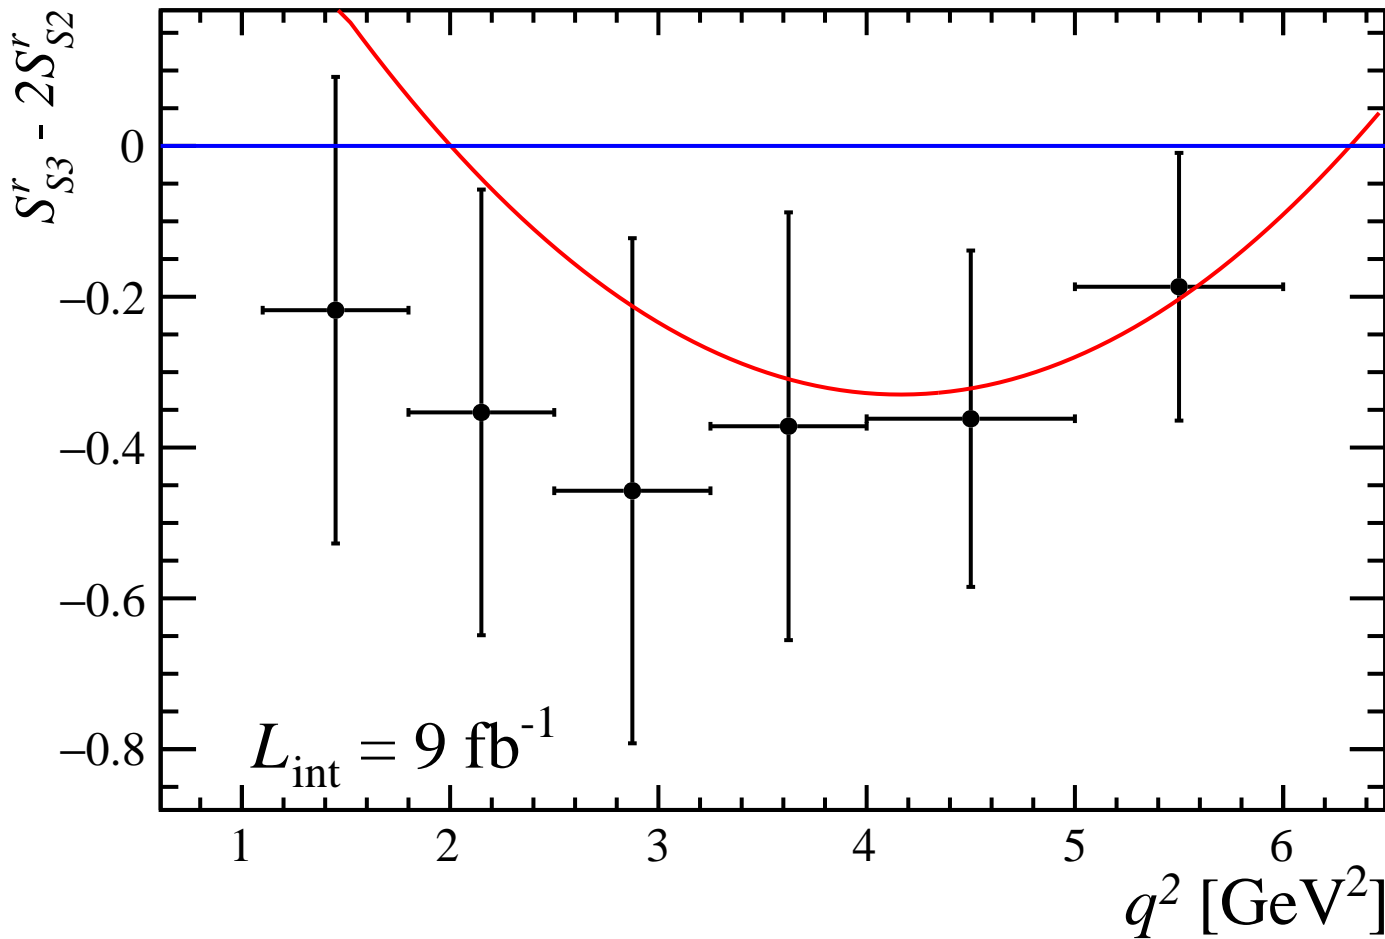

Supplement: Supplementary file 1 [file zcp_narrow_SM_run2_fits.pdf]
